# Supplementary material for: Combining ID's, Attributes, and Policies in Hyperledger Fabric
Source: arXiv:2207.01599 source file (2022-07-04)
Supplement: Supplementary file 1 [file appendix-a.tex]

\onecolumn
\appendix
\section{Search Queries}
\begin{figure}[H]
    \centering
    \includegraphics[width=0.83\textwidth]{images/Search Queries.jpg}
    \caption{Google Scholar search queries that have been used during the literature research, as described in \cite{tulib-search-plan}. First, five different search queries have been defined, which were then combined using the “AND” operator.}
\end{figure}

\section{Ledger Data Format}
\begin{figure}[H]
    \centering
    \includegraphics[width=0.83\textwidth]{images/Ledger Data.png}
    \caption{Format of the data stored on the shared blockchain ledger. The first table represents the hashmap that stores X.509 certificates, as described in Section 5.1. The second table represents the storage of application data, in this case metadata of files stored on IPFS.}
\end{figure}
\twocolumn
